# Supplementary material for: Bayesian Bi-level Sparse Group Regressions for Macroeconomic Density Forecasting
Source: arXiv:2404.02671 source file (2024-11-15)
Supplement: Supplementary file 1 [file Prior_additional_elements.tex]

%================================================================================================================================================================================================
\input{inputs/Appendix_prior_short}
%================================================================================================================================================================================================
\subsection*{Induced prior on $\varphi_j$}\label{A:sss:prior_varphi}
\indent The prior \eqref{eq:prior:dirac}-\eqref{eq:prior:b} induces a conditional prior on the random function $\varphi_j$, given $\{v_{ji}\}_{i=1}^g$ and $g$, which can be viewed as a mixture of a degenerate Gaussian process and a Dirac distribution at zero. To see this, denote $z_{j,t-h,i} := z_{ji}(\bx_{j,t-h})$ and let $\Omega_{0,j}:\mathcal{H}_j\rightarrow \mathcal{H}_j$ be a covariance operator defined as: $\forall h\in\mathcal{H}_j$, $(\Omega_{0,j}h)(\cdot) := \sum_{i=1}^g v_{ji}^2 \langle z_{ji},h \rangle z_{ji}(\cdot)$, where $\langle\cdot,\cdot\rangle$ is the inner product in $\mathcal{H}_j$. If $\mathcal{H}_j$ is an infinite dimensional space, or has dimension larger than $g$, then $\Omega_{0,j}$ is not injective and has a nontrivial null space that contains $B_{t,j}(g)$. Hence, \eqref{eq:prior:dirac}-\eqref{eq:prior:b} induce the following conditional mixture prior on the random function $\varphi_j$: for every $j\in\{1,\ldots,N\}$,
\begin{equation}
  \varphi_j|\pi_0, \{v_{ji}\}_{i=1}^g, g \sim (1 - \pi_0)\mathcal{GP}(0,\Omega_{0,j}) + \pi_0 \delta_0(\varphi_j).
\end{equation}
As $g\rightarrow \infty$, the $\mathcal{GP}(0,\Omega_{0,j})$ is a well-defined Gaussian Process in $\mathcal{H}_j$ if and only if $\Omega_{0,j}$ is a trace-class operator, that is, if $\lim_{g\rightarrow\infty}\sum_{i=1}^g v_{ji}^2 <\infty$ by assuming $\{z_{ji}\}_i$ forms an orthonormal system. Once we integrate out $v_{ji}^2$ with respect to its prior, we find that $\EE[v_{ji}^2] =\EE[\EE[v_{ji}^2|\tau_j, \pi_1]] = 3d_1\lambda_{1,j}^2/[4(c_1 + d_1)]$. So, $\Omega_{0,j}$ is a trace-class operator if $3d_1\lambda_{1,j}^2/[4(c_1 + d_1)] = \mathcal{O}(1/g)$, which is guaranteed by Assumption \ref{Ass:3} \textit{(iv)} in the main document.%\\
%================================================================================================================================================================================================
\subsection*{Modified priors}
It is worth noting that some priors defined in Section \ref{sec:priors} can be slightly, but conveniently, modified without affecting the theoretical properties discussed in Section \ref{sec:Asymptotic_Analysis}. For instance, we can allow $\pi_{1}$, which controls for the overall prior inclusion probability for the groups of coefficients, to be group-specific. In this case, we can replace $\pi_{1}$ in step \textit{(b-1)} of Algorithm 1%\ref{algorithm:1} 
with $\pi_{1,j}$, and change the conditional posterior of $\pi_{1}$ in step \textit{(e)} with:
\begin{displaymath}
\pi_{1,j} \vert \textit{rest} \sim \mathcal{B}\left(g-\sum_{i=1}^{g}\gamma_{1,ji}+c_{1},\sum_{i=1}^{g}\gamma_{1,ji}+d_{1} \right).
\end{displaymath}
Further, we can employ a hierarchical prior for the variance of the error distribution, as in \citet{Bitto2019}: $\sigma^{2}\vert a_{1} \sim \mathcal{G}^{-1} (a_{0},a_{1})$, $a_{1}\sim\mathcal{G}(e_{0},e_{1})$,
%\begin{displaymath}
%\sigma^{2}\vert a_{1} \sim \mathcal{G}^{-1} (a_{0},a_{1}) \qquad\qquad a_{1}\sim\mathcal{G}(e_{0},e_{1})
%\end{displaymath}
with hyperparameters $a_{0}$, $e_{0}$, and $e_{1}$, set to conventional values $a_{0}=2.5$, $e_{0}=5$, $e_{1}=e_{0}/(a_{0}-1)$. In this case, we extend step \textit{(a)} with the conditional posterior distribution of $a_{1}$:
\begin{displaymath}
a_{1} \vert \textit{rest} \sim \mathcal{G}\left(e_{0}+a_{0}, e_{1}+\frac{1}{\sigma^{2}}\right).
\end{displaymath}
Preliminary analysis pointed to an improvement, although marginal, of estimation results when these changes are accounted for in the MCMC sampling scheme. The modified priors are hence implemented in Algorithm 1 %\ref{algorithm:1} 
for the remainder of the paper. 
%================================================================================================================================================================================================
\subsection*{Choice of hyperparameters for implementation}
In the Monte Carlo analysis reported in Section \ref{sec:MCsim} and in the empirical application reported in Section \ref{sec:emp_app}, the hyperparameters $\lambda_{0}$ and $\lambda_{1,j}$ of the prior for $\tau_j$ are set to $\lambda_{0}=1/2$ and $\lambda_{1,j}=\log(\log(\max(N,T)))$. Both satisfy the conditions in our theoretical analysis, but other values are also compatible with our theory.
As for the hyperparameters of the priors on $\pi_{0}$ and $\pi_{1}$, their values must be chosen very carefully, as they control the overall amount of between-group and within-group prior sparsity. Assumption \ref{Ass:3} and Appendix \ref{App:hyperparam} provide conditions and guidelines for the choice of these hyperparameters. By fixing $d_{0}=d_{1}=1$, then Assumption \ref{Ass:3} \textit{(i)} - \textit{(ii)} implies that $c_{0}$ and $c_{1}$ have to satisfy the following lower-bounds: for every $N>1$,
\begin{equation}\label{eq:lower_bounds}
  c_0 \geq 1 -N + \frac{N^{u_0+1}}{k_0}, \qquad\qquad c_1 \geq 1 - Ng + \frac{(s_0^{gr}g)^{u_1} Ng}{k_1},
\end{equation}
\noindent where $k_0$ and $k_1$ are constants, and $u_0$ and $u_1$ have to belong to intervals whose bounds depend on DGP parameters $(N,s_{0}^{gr},s_{0},g)$. The non-asymptotic lower-bounds in \eqref{eq:lower_bounds} are useful in practice if optimal values for $c_0$ and $c_1$ are selected through a grid search. %given these lower-bounds, a data-driven approach can be used to fine-tune the optimal parameters.
In this paper, we propose to select $c_0$ and $c_1$ by using a data-driven approach based on the Deviance Information Criterion (DIC; \citealp{Spiegelhalter2002}), defined as:
\begin{equation}\label{eq:DIC}
\text{DIC}(\mathbf{c}|y,\bX) := -4 \mathbb{E}_{\boldsymbol\btheta,\sigma^2}\big[\log f(y\vert \boldsymbol\btheta,\sigma^2,\bX)\vert y,\bX, \mathbf{c} \big] + 2\log f(y\vert \widehat{\btheta}_{\mathbf{c}},\widehat\sigma_{\mathbf{c}}^2,\bX),
\end{equation}
where $(\btheta^{\prime}_{\mathbf{c}},\sigma^{2}_{\mathbf{c}})^{\prime}$ denotes the model parameters for a given set of hyperparameters $\mathbf{c}=(c_{0},c_{1})$, and $(\widehat{\btheta}_{\mathbf{c}},\widehat\sigma_{\mathbf{c}}^2)$ is a point estimate of $(\btheta^{\prime}_{\mathbf{c}},\sigma^{2}_{\mathbf{c}})^{\prime}$.\footnote{The first part of \eqref{eq:DIC} is the posterior mean deviance, which is here estimated by averaging the log-likelihood function, $\log  f(y\vert \btheta,\sigma^2,\bX)$, over the posterior draws of $(\btheta,\sigma^2)$. $(\widehat{\btheta}_{\mathbf{c}},\widehat\sigma_{\mathbf{c}}^2)$ is computed using the posterior median for $\btheta$ and the posterior mean for $\sigma^2$.}
This metrics of fit presents the advantage of being easily available from the Gibbs output, with no additional costs in terms of computational burden. We hence select the hyperparameters $c_{0}$ and $c_{1}$ that minimize the DIC by performing a random search on a fine 2-dimensional grid, with lower-bounds set as described in \eqref{eq:lower_bounds}. In the Monte Carlo simulations, we set the lower-bounds at the largest possible value over all the alternative DGPs considered. In this way we ensure that the selected $c_0$ and $c_1$ satisfy \eqref{eq:lower_bounds} for all the DGPs under comparison. In empirical applications, $s_{0}^{gr}$ and $s_{0}$ are unknown, but we recommend to tune them at some arbitrary values such that the inequalities in \eqref{eq:lower_bounds} are satisfied for low values of $c_{0}$ and $c_{1}$. Therefore, the price to pay for not knowing $s_{0}^{gr}$ and $s_{0}$ is simply to have to search on a larger grid. As an alternative to the DIC, one could select $c_0$ and $c_1$ by using marginal likelihood approaches \citep{Chib1995,ChibJeliazkov2001}, which are often considered in the literature for model comparison (\textit{e.g.}, Bayes factor). Our experience in our particular setting has pointed out in favour of the DIC.
